# Supplementary material for: GPU-Accelerated Mobile Multi-view Style Transfer
Source: arXiv:2003.00706 source file (2020-03-02)
Supplement: Supplementary file 1 [file AppendixA.tex]

\appendix

\subsection{Disparity-driven Multi-view Rendering} \label{multi-view synthesis}
Rendering novel views from a stereo pair is an active area of research \cite{scharstein1996stereo, avidan1997novel, avidan1998novel, martin2008fast}
This section provides a more in-depth overview of our view synthesis technique because we use our own algorithms both for CPU and GPU and rendering. Both versions implement the following general logic. Multi-view render module $\mathcal{R}$ renders a novel view from input views and disparity maps, either in single or stereo configuration, using a forward warping function $\overrightarrow{\mathcal{W}}$ and in-painting method $\mathcal{P}$ \cite{ravi2013image, oh2009hole, telea2004image}.

In the single input case, $\overrightarrow{\mathcal{W}}$ takes an image $I_a$ corresponding to viewpoint $a \in \mathbb{R}^2$ and a disparity map $\Delta_a^b$ that specifies the amount to translate each pixel in $I_a$ to where it projects in the output image $I_b$ corresponding to viewpoint $b \in \mathbb{R}^2$. The image $I_b$ is rendered so that for all $x$ such that $I_a(x)$ is visible from viewpoint $b$ we have

$$I_b(x+\Delta_a^b(x))=I_a(x)\,.$$

When the above equation has many solutions for $x$, commonly known as \emph{overdraw}, only one such pixel $I_a(x)$ can be visible, which is decided by a depth test. The depth test can be formulated as follows. For all $x_1$, if there exists $x_2$ such that $x_1+\Delta_a^b(x_1)=x_2+\Delta_a^b(x_2)$ and $$\Delta_a^b(x_2) < \Delta_a^b(x_1)\,,$$ then $I_a(x_1)$ is not visible from viewpoint $b$.

For stereo input, we extend the forward warping function $\overrightarrow{\mathcal{W}}$ to blend both input views $I_l$ and $I_r$ to produce a novel view by assigning each pixel $I_b(x)$ in the output image based on one of four cases:

\begin{enumerate}
    \item There exists $x_l$ and $x_r$ such that $I_l(x_l)$ and $I_r(x_r)$ are both visible at viewpoint $b$, and $$x=x_l+\Delta_l^b(x_l)=x_r+\Delta_r^b(x_r)\,.$$ In this case we assign $$I_b(x)=(1-\alpha)I_l(x_l)+\alpha I_r(x_r)\,,$$ where $$\alpha=\begin{cases} 
          0 & b < l\\
          1 & b > r \\
          \frac{b-l}{r-l} & l<b<r 
       \end{cases}$$
    \item There exists $x_l$ such that $I_l(x_l)$ is visible at viewpoint $b$ and $x=x_l+\Delta_l^b(x_l)$, while no $x_r$ satisfies $x=x_r+\Delta_r^b(x_r)$. Then we assign $I_b(x)=I_l(x_l)$.
    \item Same as case (2), exchanging $l$ and $r$.
    \item No $x_l$ satisfies $x=x_l+\Delta_l^b(x_l)$ and no $x_r$ satisfies $x=x_r+\Delta_r^b(x_r)$. Then $I_b(x)$ remains to be in-painted by $\mathcal{P}$.
\end{enumerate}

In both the single input and stereo input scenarios, there are pixels in the output view $I_b$ that do not receive any forward warped pixels. These \emph{deoccluded} pixels are in-painted using any method $\mathcal{P}$. Our implementation involves reflecting patches of the image adjacent to a deoccluded region into the region. This is an inexpensive way to have textures continue into deoccluded regions without blurring.
